# Supplementary material for: Solvent-cosolvent attraction is sufficient to induce polymer collapse in good solvent mixtures
Source: arXiv:2410.02211 ancillary file (2024-10-04)
Supplement: Supplementary file 1 [file Supp.pdf]

## Supporting Information

### Solvent-cosolvent attraction is sufficient to induce polymer collapse in good solvent mixtures

Hitesh Garg,<sup>1,2,\*</sup> Divya Nayar,<sup>3,†</sup> and Satyavani Vemparala<sup>1,2,‡</sup>

<sup>1</sup>*The Institute of Mathematical Sciences, C.I.T. Campus, Taramani, Chennai 600113, India*

<sup>2</sup>*Homi Bhabha National Institute, Training School Complex, Anushakti Nagar, Mumbai, 400094, India*

<sup>3</sup>*Department of Material Science and Engineering, Indian Institute of Technology, Delhi, India*

(Dated: October 2, 2024)

---

\* hiteshgarg@imsc.res.in

† divyanayar@mse.iitd.ac.in

‡ vani@imsc.res.in

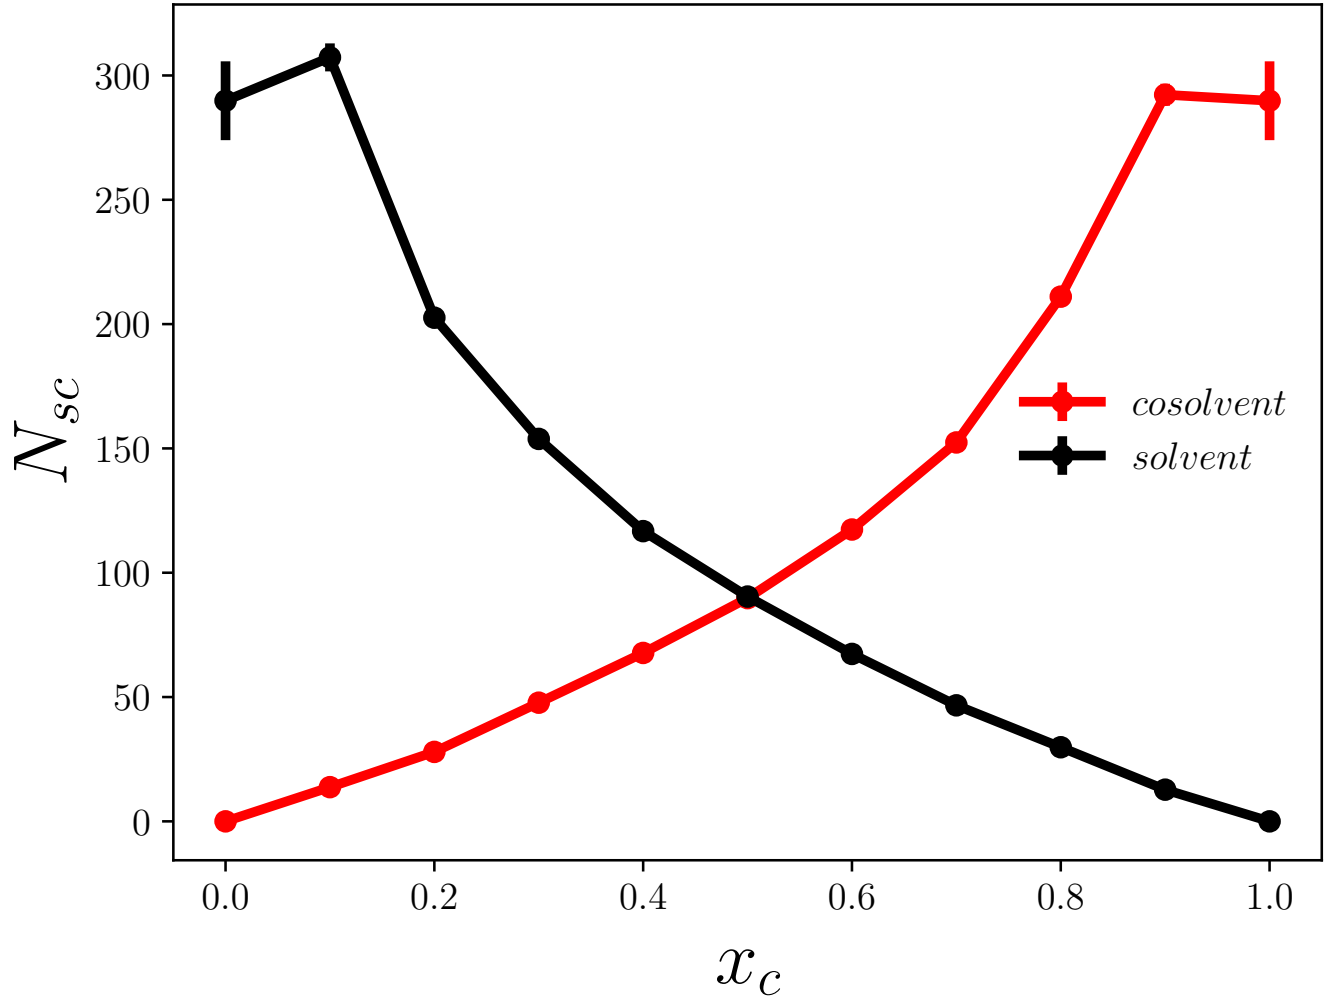

FIG. S1. Number of solvents and cosolvents in contact with polymer within  $1.5\sigma_s$  of the chain backbone

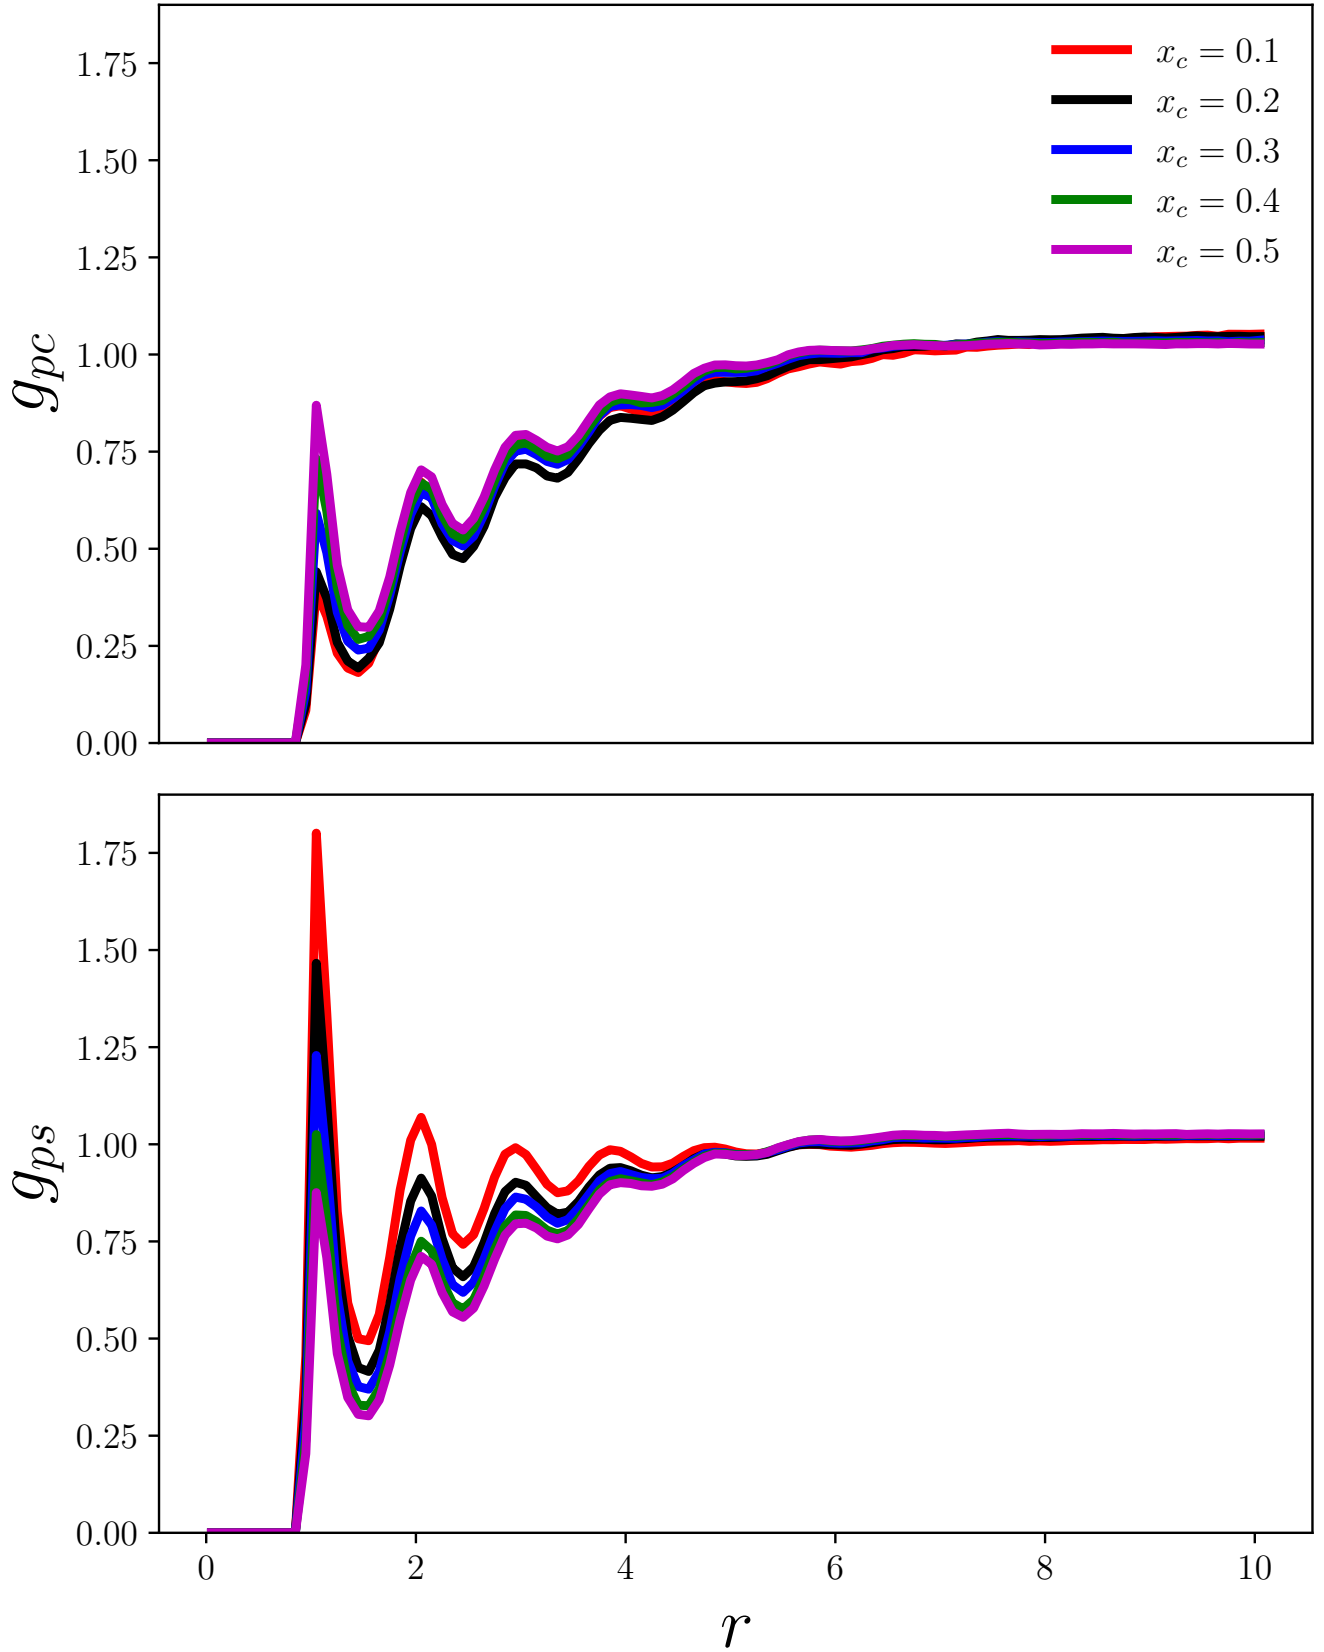

FIG. S2. Radial distribution function  $g(r)$  between polymer & cosolvent (above) and polymer & solvent (below).

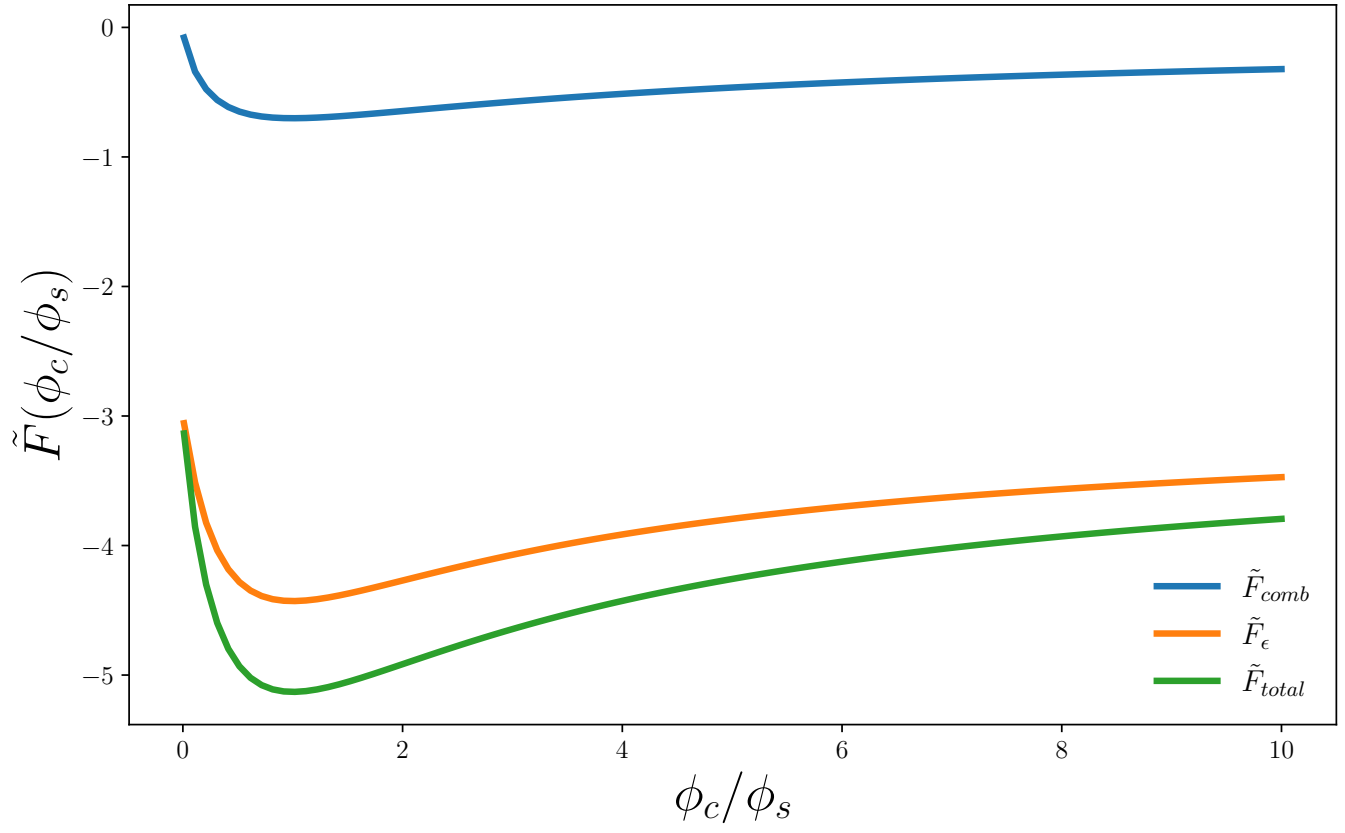

FIG. S3. The free energy from Flory-Huggins theory with ternary mixture

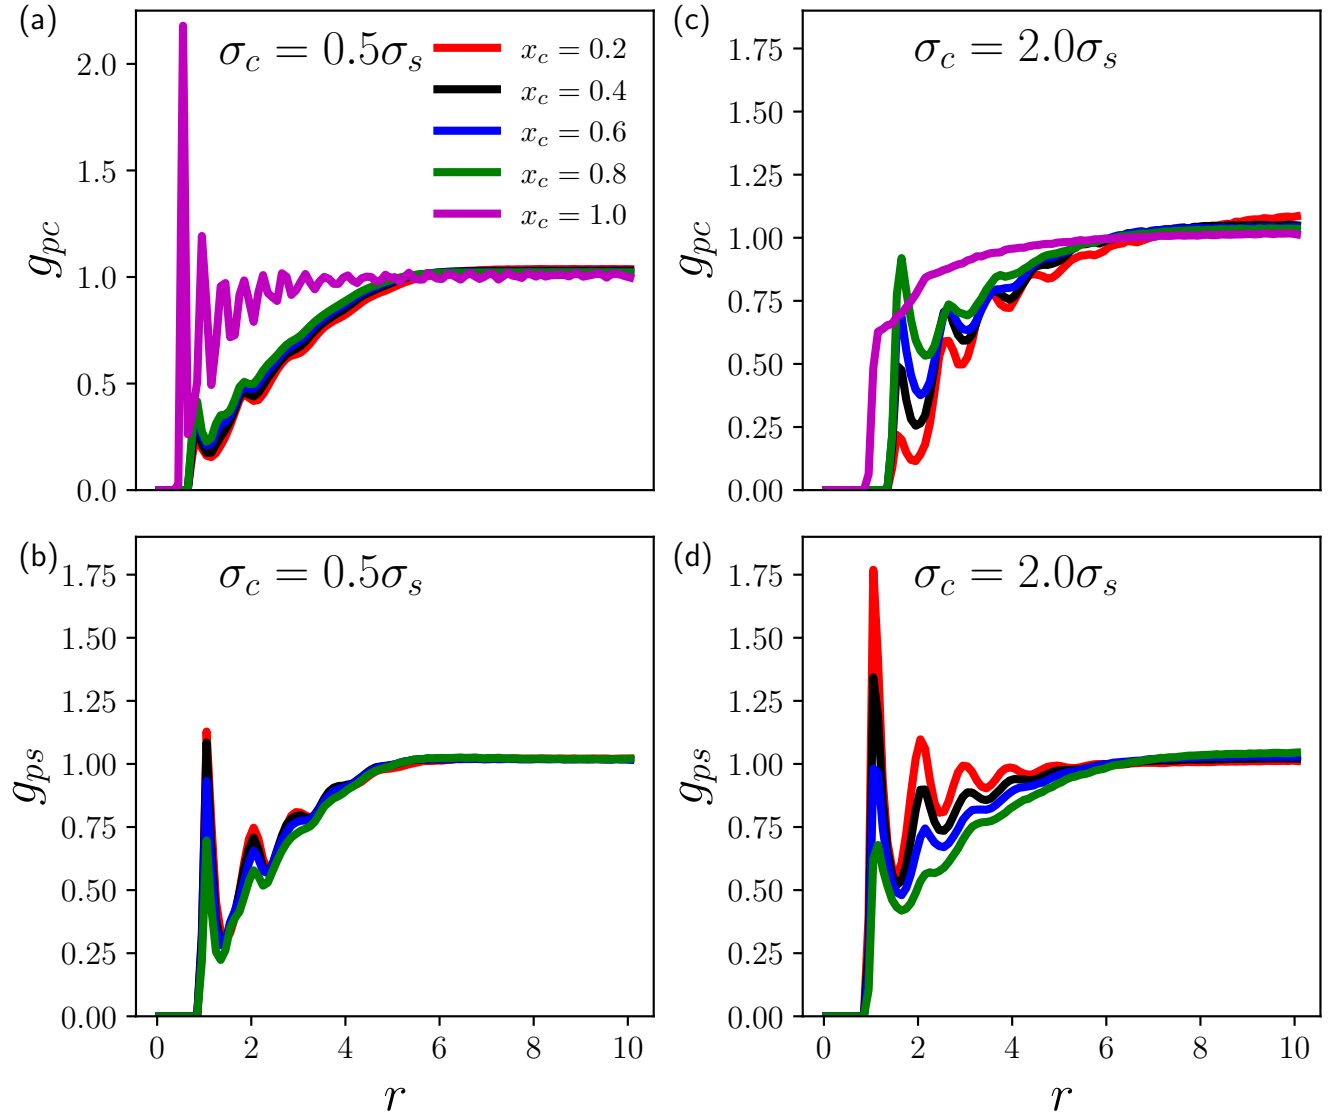

FIG. S4. Radial distribution function  $g(r)$  between (a) polymer & cosolvent for  $\sigma_A = 0.5\sigma_s$  (b) polymer & solvent for  $\sigma_A = 0.5\sigma_s$  (c) polymer & cosolvent for  $\sigma_A = 2.0\sigma_s$  (d) polymer & solvent for  $\sigma_A = 2.0\sigma_s$ .

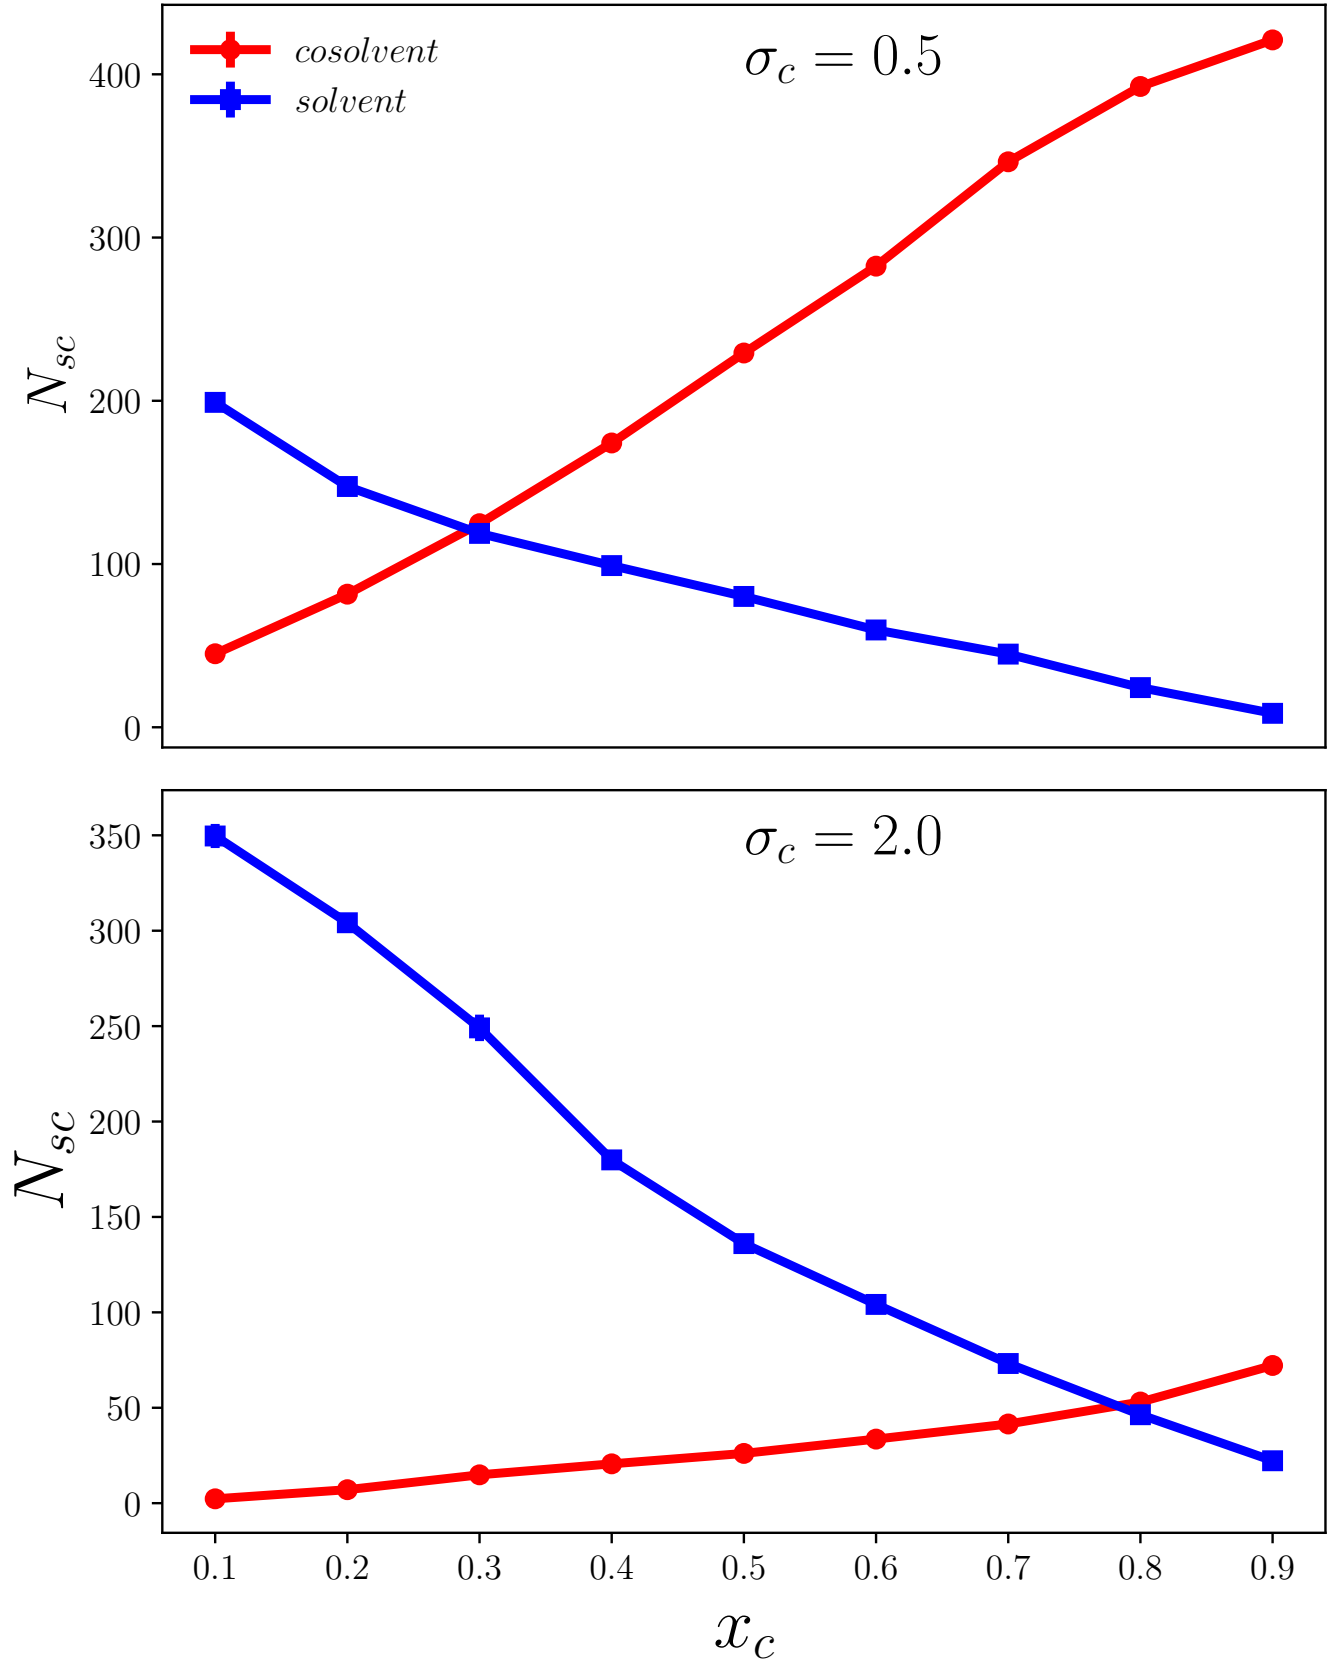

FIG. S5. Number of solvents/cosolvents in contact with polymer within  $1.5\sigma_s$  of chain backbone for  $\sigma_c = 0.5\sigma_s$  (above) and  $\sigma_c = 2.0\sigma_s$  (below)
